# Supplementary material for: Insider Stories: Analyzing Internal Sustainability Efforts of Major US Companies from Online Reviews
Source: arXiv:2205.01217 source file (2023-04-13)
Supplement: Supplementary file 2 [file obsolete.tex]

\begin{comment}


% Table created by stargazer v.5.2.2 by Marek Hlavac, Harvard University. E-mail: hlavac at fas.harvard.edu
% Date and time: Fri, Jul 09, 2021 - 09:11:23 AM
% Requires LaTeX packages: dcolumn 
\begin{table*}[t] \centering \scriptsize
  \caption{Linear regressions.}
  \label{table:6goals} 
\begin{tabular}{@{\extracolsep{-30pt}}lD{.}{.}{-3} D{.}{.}{-3} D{.}{.}{-3} D{.}{.}{-3} D{.}{.}{-3} D{.}{.}{-3} } 
\\[-1.8ex]\hline 
\hline \\[-1.8ex] 
 & \multicolumn{6}{c}{\textit{Dependent variable:}} \\ 
\cline{2-7} 
\\[-1.8ex] & \multicolumn{6}{c}{State-level} \\ 
 & \multicolumn{1}{c}{Health} & \multicolumn{1}{c}{Education} & \multicolumn{1}{c}{Gender equ } & \multicolumn{1}{c}{Financial} & \multicolumn{1}{c}{Support Inf} & \multicolumn{1}{c}{Support Env} \\
\\[-1.8ex] & \multicolumn{1}{c}{(1)} & \multicolumn{1}{c}{(2)} & \multicolumn{1}{c}{(3)} & \multicolumn{1}{c}{(4)} & \multicolumn{1}{c}{(5)} & \multicolumn{1}{c}{(6)}\\ 
\hline \\[-1.8ex] 
 % $S(u)$ &  &  &  & -0.089^{**}$ $(0.044) &  &  \\ 
    log(\#reviews) &  &  &  & -0.089^{**}$ $(0.044) &  &  \\ 
    log(population) &  &  &  & -0.089^{**}$ $(0.044) &  &  \\ 
    log(\#reviews)* log(population) &  &  &  & -0.089^{**}$ $(0.044) &  &  \\ 
 Neuroticism & -0.113^{***}$ $(0.038) &  &  & -0.098^{*}$ $(0.049) & -0.060^{**}$ $(0.027) &  \\ 
Agreeableness &  &  &  &  &  & 0.039^{*}$ $(0.020) \\ 
%   SOCIOECONOMIC\_no\_high\_school\_diploma &  & -0.110^{***}$ $(0.037) &  &  &  & -0.055^{**}$ $(0.025) \\ 
  Cultural Tightness &  &  &  & 0.062$ $(0.044) &  &  \\ 
%   SOCIOECONOMIC\_population\_2019 & 0.092^{***}$ $(0.034) & 0.102^{**}$ $(0.039) & 0.103^{***}$ $(0.030) & 0.051$ $(0.033) & 0.046^{*}$ $(0.023) & 0.042^{*}$ $(0.021) \\ 
%   SOCIOECONOMIC\_density\_2015 &  & -0.069$ $(0.044) &  & -0.027$ $(0.039) &  &  \\ 
%   POLITICAL\_p\_ideo\_diff & -0.187^{***}$ $(0.046) & -0.120^{*}$ $(0.062) & -0.091^{**}$ $(0.039) & -0.111^{*}$ $(0.065) &  &  \\ 
%   population\_2019:\_density\_2015 &  &  &  & -0.096^{*}$ $(0.052) &  &  \\ 
%   SOCIOECONOMIC\_gdp\_per\_capita\_2017 &  &  &  &  &  & -0.075$ $(0.055) \\ 
%   Constant & 0.542^{***}$ $(0.030) & 0.563^{***}$ $(0.036) & 0.519^{***}$ $(0.029) & 0.532^{***}$ $(0.031) & 0.489^{***}$ $(0.024) & 0.491^{***}$ $(0.020) \\ 
 \hline \\[-1.8ex] 
Observations & \multicolumn{1}{c}{43} & \multicolumn{1}{c}{43} & \multicolumn{1}{c}{43} & \multicolumn{1}{c}{43} & \multicolumn{1}{c}{43} & \multicolumn{1}{c}{43} \\ 
R$^{2}$ & \multicolumn{1}{c}{0.568} & \multicolumn{1}{c}{0.372} & \multicolumn{1}{c}{0.398} & \multicolumn{1}{c}{0.351} & \multicolumn{1}{c}{0.282} & \multicolumn{1}{c}{0.204} \\ 
Adjusted R$^{2}$ & \multicolumn{1}{c}{0.523} & \multicolumn{1}{c}{0.306} & \multicolumn{1}{c}{0.368} & \multicolumn{1}{c}{0.221} & \multicolumn{1}{c}{0.227} & \multicolumn{1}{c}{0.120} \\ 
Residual Std. Error & \multicolumn{1}{c}{0.192 (df = 38)} & \multicolumn{1}{c}{0.222 (df = 38)} & \multicolumn{1}{c}{0.187 (df = 40)} & \multicolumn{1}{c}{0.185 (df = 35)} & \multicolumn{1}{c}{0.151 (df = 39)} & \multicolumn{1}{c}{0.119 (df = 38)} \\ 
F Statistic & \multicolumn{1}{c}{12.516$^{***}$ (df = 4; 38)} & \multicolumn{1}{c}{5.629$^{***}$ (df = 4; 38)} & \multicolumn{1}{c}{13.206$^{***}$ (df = 2; 40)} & \multicolumn{1}{c}{2.699$^{**}$ (df = 7; 35)} & \multicolumn{1}{c}{5.117$^{***}$ (df = 3; 39)} & \multicolumn{1}{c}{2.432$^{*}$ (df = 4; 38)} \\ 
\hline 
\hline \\[-1.8ex] 
\textit{Note:}  & \multicolumn{6}{r}{$^{*}$p$<$0.1; $^{**}$p$<$0.05; $^{***}$p$<$0.01} \\ 
\end{tabular} 
\end{table*} 
\end{comment}
