# Supplementary material for: Insider Stories: Analyzing Internal Sustainability Efforts of Major US Companies from Online Reviews
Source: arXiv:2205.01217 source file (2023-04-13)
Supplement: Supplementary file 3 [file supplementary_old.tex]

\documentclass[10pt]{amsart}

\usepackage{geometry}
\geometry{paperheight=11in,
          paperwidth=8.5in,
          left=2cm, right=2cm, top=2cm, bottom=2cm
         }
\usepackage{parskip}

\usepackage{graphicx}
\usepackage{amssymb}
\usepackage{epstopdf}
\usepackage{url}
\usepackage{subfigure}
\usepackage{lineno}
\usepackage{color}

\usepackage[foot]{amsaddr}
\usepackage{placeins}
\usepackage{mathtools}
\usepackage{color, colortbl}
\usepackage{fancyhdr}
\usepackage{ctable}
\definecolor{Gray}{gray}{0.9}
\usepackage{enumitem}
\usepackage{graphicx}
\usepackage{caption}
\usepackage{color, colortbl}
\usepackage{array}
\usepackage{booktabs} % For formal tables
\usepackage{makecell}
\usepackage{cellspace}
\usepackage{tabularx}
\usepackage{multirow}
\usepackage{natbib}
\usepackage{comment}

\newcommand\todo[1]{\textcolor{red}{[#1]}}
\newcommand{\rev}[1]{\textcolor{blue}{#1}}


\begin{document}


\title[Corporate Sustainability]{Insider Stories\\Supplementary Information}


% \author{Luca Maria Aiello$^{1,2}$}
% \author{Daniele Quercia$^{1,3,*}$}
% \author{Ke Zhou$^{1}$}
% \author{Marios Constantinides$^{1}$}
% \author{Sanja Scepanovic$^{1}$}
% \author{Sagar Joglekar$^{1}$}


% \address{$^{1}$Nokia Bell Labs Cambridge, United Kingdom}
% \address{$^{2}$IT University Copenhagen, Denmark}
% \address{$^{3}$CUSP, King's College London, United Kingdom}
% \address{$^{*}$Corresponding author: quercia@cantab.net}

\flushbottom
\maketitle
\thispagestyle{empty}


% \begin{figure*}[h!]
%     \centering
%     \includegraphics[width=0.65\linewidth]{figure/representativeness_time_num_posts.png}
%     \caption{Number of posts (log) in our dataset between 2008 and 2020s. There is no trend difference between all posts and those containing mentions related to stress.}
%     \label{fig:supp-temporal_reviews}
% \end{figure*}

\section*{Details of the dataset}
We collected a total of 713,018 posts published for a company reviewing site from the start of 2008 up until the first quarter of 2020 for the S\&P 500 companies. We filtered out posts belonging to non-US based companies, yielding a total of 439,163 posts across $399$ unique S\&P 500 companies. The average rating across companies ranged from a minimum value of $1.62$ up to a maximum value of $5$ ($ \mu = 3.37, \sigma = 0.40)$. While the overall fraction of stress posts per company was $1.11\%$, this value ranged from $0\%$ up to $9.52\%$ across companies ($ \mu = 1\%, \sigma = 1\%)$.

\section*{Data Representativeness}

A total of 439,163 posts were analyzed. These posts are about companies distributed across all  the 51 U.S. states (Table~\ref{tabsup:posts_states}). The highest number of  posts were found in California (i.e., a total of 69,968 posts), while the lowest in Wyoming (i.e., a total of 222 posts). The posts span across 11 industries classified according to the Global Industry Classification Standard (GICS), with the highest number of posts for companies in Information Technology, and the least number in Real Estate (Table~\ref{tabsup:industries}). The posts were written by managers, sales associates, software engineers, analysts, among others (Table~\ref{tabsup:employees_titles}). The maximum annual number of posts between 2008 and 2020 was observed in 2016, while the lowest number of posts in 2009. 




\begin{table}[!htb]
\caption{Number of posts and number of offices on the company reviewing site across U.S. States, ranked by the number of posts published between 2008 and 2020 in descending order. The state of California had the most published posts, while the state of Wyoming had the least published posts. The Pearson correlation between the log number of posts and the number of companies per state in our data is $.98$, while the correlation between the log number of posts in our data and the log of population size across states is $.93$.}
\label{tabsup:posts_states}
\begin{minipage}{0.5\textwidth}
\centering
\begin{tabular}{ccc}
\toprule
\textbf{U.S. State} & \textbf{\# posts} & \textbf{\# offices} \\
\midrule
   CA &              69968 &      340 \\
   TX &              43629 &      342 \\
   NY &              37515 &      313 \\
   IL &              25157 &      290 \\
   FL &              24082 &      283 \\
   GA &              17888 &      275 \\
   WA &              15672 &      239 \\
   NC &              14072 &      268 \\
   PA &              14064 &      271 \\
   OH &              12447 &      263 \\
   MA &              12355 &      253 \\
   AZ &              11834 &      228 \\
   NJ &              11561 &      245 \\
   VA &              11320 &      235 \\
   CO &               9408 &      249 \\
   MN &               8437 &      196 \\
   MI &               7953 &      237 \\
   MO &               7657 &      230 \\
   TN &               7165 &      221 \\
   OR &               6704 &      206 \\
   MD &               6610 &      207 \\
   IN &               5727 &      222 \\
   WI &               5006 &      181 \\
   CT &               4567 &      186 \\
   KY &               4224 &      190 \\
   UT &               3925 &      187 \\
% \bottomrule
% \end{tabular}



% \end{minipage} \hfill
% \begin{minipage}{0.5\textwidth}
% \begin{tabular}{ccc}
% \toprule
% \textbf{U.S. State} & \textbf{\# posts} & \textbf{\# offices} \\
% \midrule
   OK &               3772 &      174 \\
   DC &               3596 &      180 \\
   KS &               3459 &      169 \\
   SC &               3362 &      194 \\
   NV &               2815 &      163 \\
   LA &               2631 &      175 \\
   AL &               2546 &      171 \\
   DE &               2067 &      113 \\
   IA &               1849 &      133 \\
   RI &               1676 &      103 \\
   AR &               1666 &      149 \\
   NH &               1627 &      127 \\
   NE &               1564 &      139 \\
   ID &               1208 &      112 \\
   MS &               1138 &      127 \\
   NM &               1097 &      125 \\
   WV &                803 &      114 \\
   ME &                604 &      105 \\
   HI &                600 &       85 \\
   ND &                344 &       74 \\
   VT &                324 &       54 \\
   MT &                322 &       70 \\
   AK &                300 &       57 \\
   SD &                297 &       57 \\
   WY &                222 &       72 \\
    &                 &        \\
\bottomrule
\end{tabular}
\end{minipage}
\end{table}

\begin{figure*}
    \centering
    \includegraphics[width=0.55\linewidth]{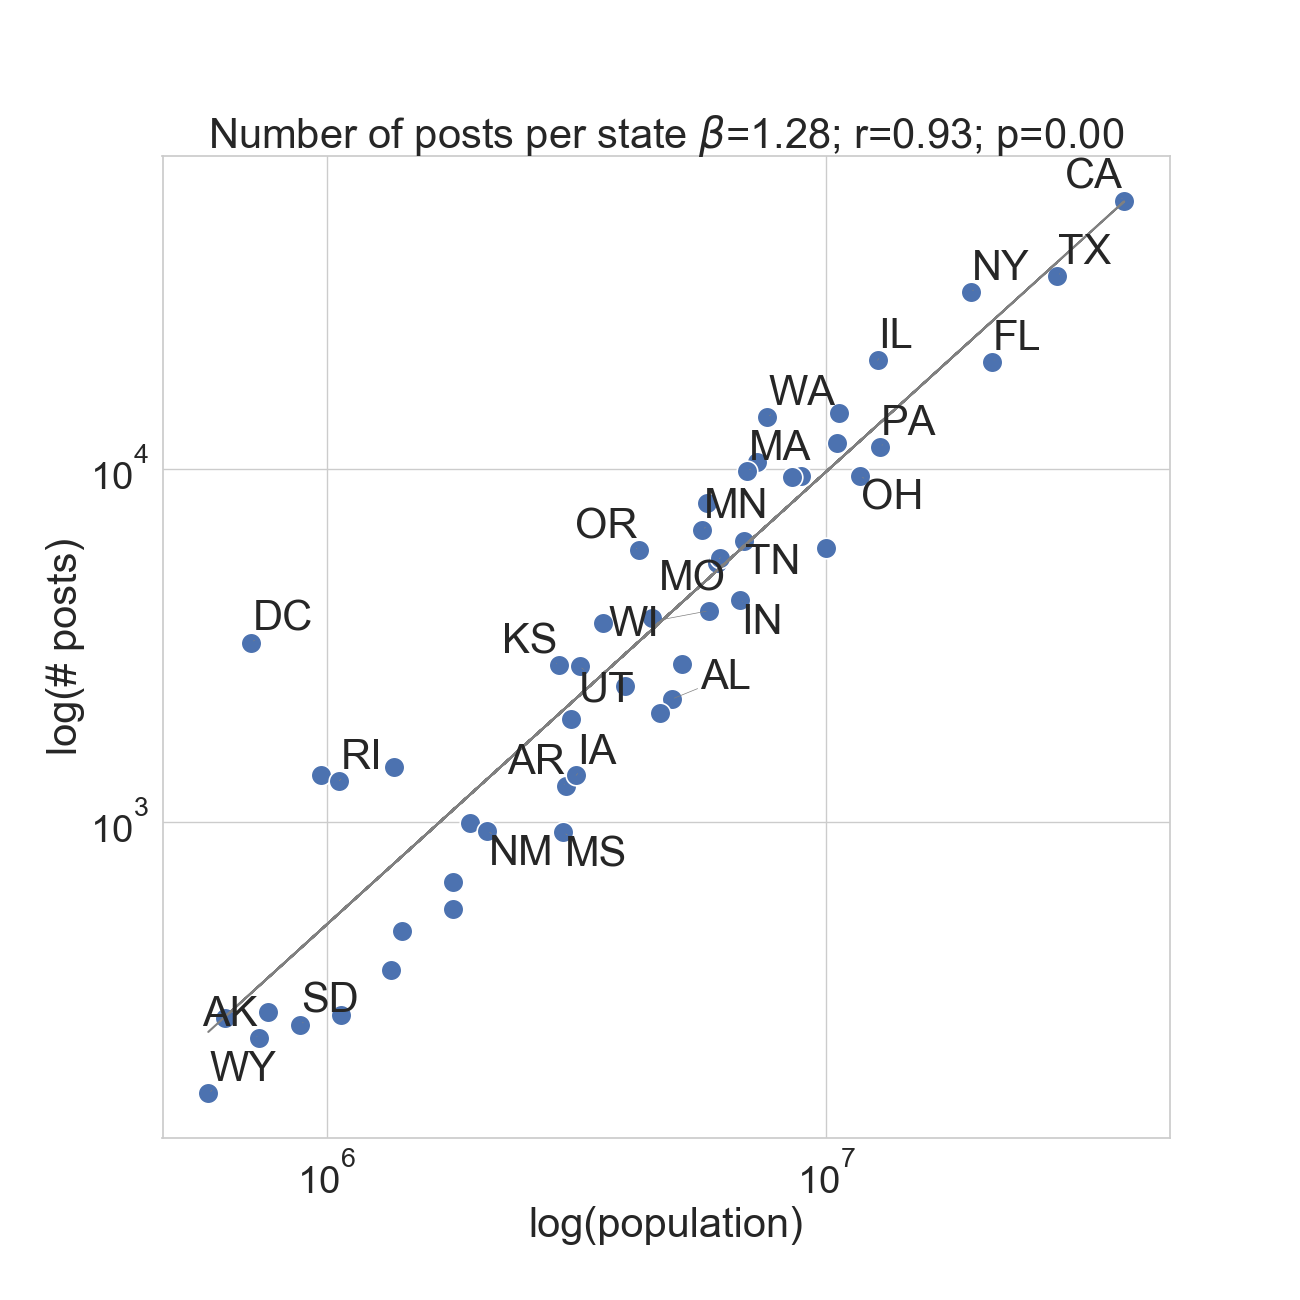}
    \caption{Number of posts (log) in our dataset versus state population (log). The  states Washington DC and Rhode Island have more posts that what the population size would suggest. The line of best linear fit is shown in gray. U.S. states are shown with the two-code state abbreviation.}
    \label{fig:supp-spatial_rep}
\end{figure*}




\begin{table}[t!]
\caption{Number of posts across the Global Industry Classification Standard (GICS) sectors. More posts are generally found in sectors having more companies, as one expects.}
\label{tabsup:industries}
\centering
\begin{tabular}{lrr}
\toprule \textbf{GICS Sector} &  \textbf{\# posts} &  \textbf{\# companies} \\
\midrule
 Information Technology &              63198 &         52 \\
 Consumer Discretionary &              62395 &         40 \\
             Financials &              49955 &         42 \\
            Health Care &              36308 &         41 \\
       Consumer Staples &              26471 &         28 \\
            Industrials &              24074 &         43 \\
 Communication Services &              13842 &         13 \\
                 Energy &               5510 &         20 \\
              Materials &               5269 &         21 \\
              Utilities &               3172 &         19 \\
            Real Estate &               2228 &         16 \\
\bottomrule
\end{tabular}
\end{table}

\begin{table}[t!]
\caption{Number of posts across roles and statuses.}
\label{tabsup:employees_titles}
\centering
\begin{tabular}{lr}
\toprule \textbf{Employee Title} &  \textbf{\# posts} \\
\midrule
                  Sales Associate &        8006 \\
                          Manager &        4536 \\
                Software Engineer &        4191 \\
  Customer Service Representative &        4058 \\
                          Cashier &        3726 \\
                         Director &        2819 \\
                  Project Manager &        2365 \\
                   Senior Manager &        2225 \\
         Senior Software Engineer &        2019 \\
                        Associate &        1969 \\
                    Store Manager &        1963 \\
                Assistant Manager &        1930 \\
              Pharmacy Technician &        1747 \\
                          Analyst &        1660 \\
                  Delivery Driver &        1619 \\
\toprule \textbf{Employee Status} &  \textbf{\# posts} \\
\midrule
  Current Employee  &      181078 \\
    Current Intern  &        2789 \\
   Former Employee  &      137567 \\
 Former Contractor  &        3183 \\
     Former Intern  &        5020 \\
\bottomrule
\end{tabular}
\end{table}

\begin{figure*}
    \centering
    \includegraphics[width=0.45\linewidth]{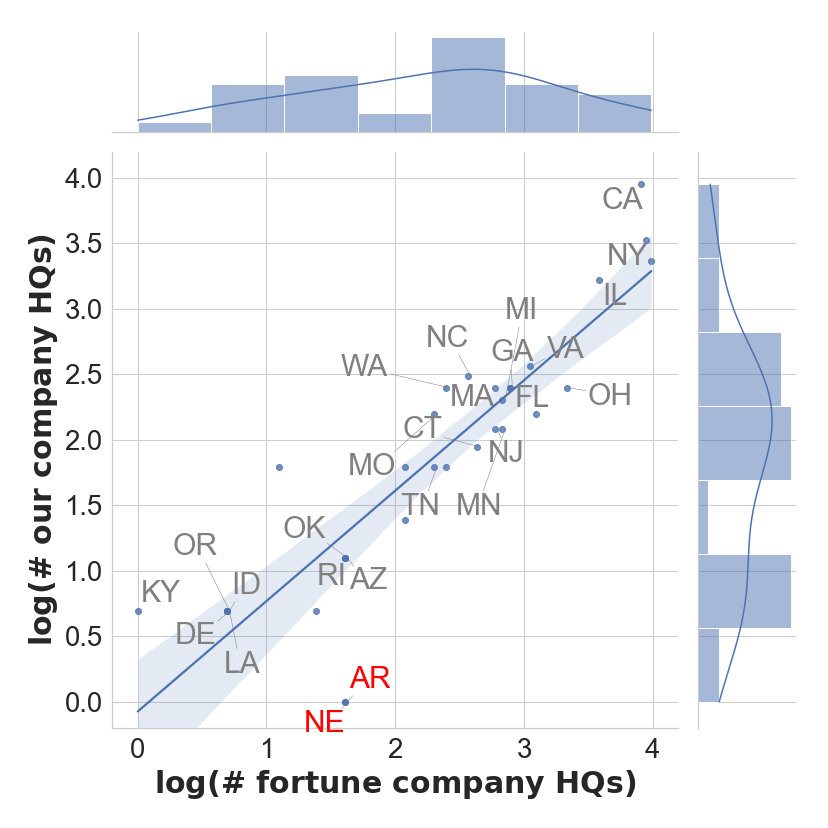}
    \caption{Correlation between the number of headquarters in each state in the Fortune 500 list and the number of headquarters in each state in our dataset (Spearman $r=.90$). The states of Nebraska (NE) and Arizona (AR) have fewer headquarters than what the Fortune list would suggests. 
    %\todo{1. please report the states of DE and DC on the dots. 2. don't color KY and MD in red as they are above the line, and mark only NE as an outlier; 3. why we used fortune 500?}
    }
    \label{fig:supp-headquarters}
\end{figure*}






\clearpage
\section{Methodological Details of our Approach for Detecting ISEs}

Here we provide a more detailed explanation of our mixed-method approach in operationalizing sustainability in the corporate context by leveraging the UN SDGs (Table~\ref{tab:defs}).

%\subsection*{Selecting sustainability goals in the corporate context}\label{sec:selecting_sdgs}
\subsection*{Step 1 - Human-driven pre-selection of goals}\label{sec:selecting_sdgs}

% from the UN \todo{explain how we got the sdg definitions}

%\comments{just copied content from Wikipedia for now.}

The Sustainable Development Goals (SDGs) or Global Goals are a collection of 17 interlinked global goals designed to be a ``blueprint to achieve a better and more sustainable future for all". The SDGs were set up in 2015 by the United Nations General Assembly and are intended to be achieved by the year 2030. They are included in a UN Resolution called the 2030 Agenda or what is colloquially known as Agenda 2030. 

The 17 SDGs are: (1) No Poverty, (2) Zero Hunger, (3) Good Health and Well-being, (4) Quality Education, (5) Gender Equality, (6) Clean Water and Sanitation, (7) Affordable and Clean Energy, (8) Decent Work and Economic Growth, (9) Industry, Innovation and Infrastructure, (10) Reducing Inequality, (11) Sustainable Cities and Communities, (12) Responsible Consumption and Production, (13) Climate Action, (14) Life Below Water, (15) Life On Land, (16) Peace, Justice, and Strong Institutions, (17) Partnerships for the Goals. 

Not all UN goals might be relevant in terms of internal corporate practice. To decide whether to completely discard some UN SDGs, three independent annotators qualitatively assessed each of the 17 goal's definition put forth by the UN. They unanimously decided to discard the following four: `life below water', `life on land', `sustainable cities', and `partnerships for goals'. More precisely, `life below water', `life on land', `sustainable cities' mainly concern the health of water bodies, land conservation, and cities, respectively. Unless one works at a company that heavily interacts with water bodies, land conservation, or cities, they would not mention these goals. `Partnership on goals', on the other hand, was explicitly designed to foster collaboration between countries to facilitate sustainability. Since, we focus entirely on US-based companies, we also exclude any goals that pertain to international co-operations.
%\notelc{add similar explanations for the other 3 we dropped}. 
At the end of this qualitative step, we were left with 13 UN SDGs to work with in the next step.


\subsection*{Step 2 - Unsupervised discovery of relevant reviews and goals}\label{sec:method}


% Please add the following required packages to your document preamble:
% \usepackage{booktabs}
% \usepackage[table,xcdraw]{xcolor}
% If you use beamer only pass "xcolor=table" option, i.e. \documentclass[xcolor=table]{beamer}
% \usepackage[normalem]{ulem}
% \useunder{\uline}{\ul}{}
\begin{table}[]
\centering
\small
\begin{tabular}{@{}
>{\columncolor[HTML]{FFFFFF}}l 
>{\columncolor[HTML]{FFFFFF}}l 
>{\columncolor[HTML]{FFFFFF}}l @{}}
\toprule
id    & Goal                                     & Definition                                                                                                                                                                                                                                \\ \midrule
SDG1  & no poverty                               & to end poverty in all its forms, everywhere                                                                                                                                                                                               \\
SDG2  & zero hunger                              & \begin{tabular}[c]{@{}l@{}}End hunger, achieve food security and improved nutrition\\  and promote sustainable agriculture\end{tabular}                                                                                                   \\
SDG3  & \textbf{good health and wellbeing}                & To ensure healthy lives and promote well-being for all at all ages.                                                                                                                                                                       \\
SDG4  & \textbf{quality education}                        & \begin{tabular}[c]{@{}l@{}}Ensure inclusive and equitable quality education and promote\\ lifelong learning opportunities for all\end{tabular}                                                                                            \\
SDG5  & \textbf{gender equality}                          & Achieve gender equality and empower all women and girls                                                                                                                                                                                   \\
SDG6  & clean water and sanitation               & \begin{tabular}[c]{@{}l@{}}Ensure availability and sustainable management of water and\\ sanitation for all.\end{tabular}                                                                                                                 \\
SDG7  & affordable and clean energy              & \begin{tabular}[c]{@{}l@{}}Ensure access to affordable, reliable, sustainable and modern\\ energy for all.\end{tabular}                                                                                                                   \\
SDG8  & \textbf{decent work and economic growth}          & \begin{tabular}[c]{@{}l@{}}Foster sustained, inclusive and sustainable economic growth,\\  full and productive employment and decent work for all.\end{tabular}                                                                           \\
SDG9  & \textbf{industry, innovation, and infrastructure} & \begin{tabular}[c]{@{}l@{}}build resilient infrastructure, promote sustainable industrialization\\ and foster innovation\end{tabular}                                                                                                     \\
SDG10 & reducing inequality                      & Reduce inequality within and among countries                                                                                                                                                                                              \\
SDG11 & sustainable cities and communities       & Make cities inclusive, safe, resilient and sustainable                                                                                                                                                                                    \\
SDG12 & responsible consumption and production   & To ensure sustainable consumption and production patterns                                                                                                                                                                                 \\
SDG13 & climate action                           & Take urgent action to combat climate change and its impacts                                                                                                                                                                               \\
SDG14 & life below water                         & \begin{tabular}[c]{@{}l@{}}Conserve and sustainably use the oceans, seas and marine resources\\ for sustainable development\end{tabular}                                                                                                  \\
SDG15 & life on land                             & \begin{tabular}[c]{@{}l@{}}Protect, restore and promote sustainable use of terrestrial\\ ecosystems, sustainably manage forests, combat desertification, \\ and halt and reverse land degradation and halt biodiversity loss\end{tabular} \\
SDG16 & \textbf{peace, justice, and strong institutions}   & \begin{tabular}[c]{@{}l@{}}Promote peaceful and inclusive societies for sustainable\\ development, provide access to justice for all and build effective,\\ accountable and inclusive institutions at all levels\end{tabular}             \\
SDG17 & partnerships for the goals               & \begin{tabular}[c]{@{}l@{}}Strengthen the means of implementation and revitalize the global\\ partnership for sustainable development\end{tabular}                                                                                        \\ \bottomrule
\end{tabular}
\caption{The 17 UN Sustainability Development Goals (SDGs) and their definitions as put forth by the UN\cite{}. The 6 goals in bold (SDGs 3,4,5,8,9, and 16) became our final 6 ISEs.}
\label{tab:defs}
\end{table}

We obtained mentions of similarity in reviews by seeing how semantically related the review sentences are to the definitions of the remaining 13 SDG goals. To find the similarity between reviews and goal definitions, we made use of a deep learning based method that is tailored to find the similarity between two sentences --- specifically, sentence BERT or s-BERT~\cite{reimers2019sentence}. BERT or Bidirectional Encoder Representations from Transformers~\cite{devlin2018bert}, and its variants like RoBERTa and DistilBERT, is a family of state-of-the-art Natural Language Processing (NLP) methods that are trained on a vast corpora of data, enabling them to learn many different types of language phenomena. One such phenomenon is semantic similarity between different sentences. s-BERT is trained especially for this task and has achieved state-of-the-art results in text similarity NLP tasks~\cite{reimers2019sentence}.

We embedded each of the 13 UN SDG definitions (Table~\ref{tab:defs}) using s-BERT to obtain 13 vectors of length 726 ($v_g$). Recall that a review consists of a title, pro and con. Therefore, we obtained sentences in each review ($p$) and embed them using S-BERT as well, to obtain the review sentence embeddings ($v_p$). Finally, we found the cosine similarity between $v_p$ and $v_g$. 

We ended up with similarity scores between -1 and 1 for all sentences for all 13 goals. The distribution of the scores is described is summarized in Figure~\ref{fig:sim_dist}. The similarity distributions are different for different goals --- `decent work' has higher average similarity compared to `gender equality'. \textcolor{blue}{To ensure high precision while accounting for the fact that the mean and range of similarity is variable for different goals, we opted for a two-step selection procedure. To shortlist reviews we followed an approach based on previous literature~\cite{das2020modeling}. First, we only selected sentences relevant to a particular goal as those which are in the 95th percentile for that goal. Then, to reduce the inclusion of reviews that were not relevant due to different similarity distributions for different goals, we selected a threshold of the average of the 95th percentile similarity for all goals (around 0.3 in this case).}

\textcolor{blue}{In addition to the threshold for reviews, we also considered whether to use pros, cons, or both for understanding ISEs. As sustainability is not a neutral concept but a positive one, and we hypothesized company-led efforts on sustainability would be appreciated or brought up more frequently in pros rather than cons. In our analysis, we found that the average similarity for pros was much higher than the average for cons (Table~\ref{tab:pros_vs_cons}), indicating that our NLP method was better at assessing sustainability concerns for pros better than for cons
%, in line with previous work demonstrating positivity bias in NLP methods~\cite{ribeiro2016sentibench}. 
This was also confirmed with qualitative analysis where 3 independent annotators assessed the top most similar cons and found them to not be relevant to the ISE they were picked for (Fleiss $k$ = 0.91). Finally, the proportion of shortlisted review for cons were much lower than those shortlisted by pros (Table~\ref{tab:pros_vs_cons}).  Therefore, having established that pros are more appropriate for understanding ISEs conceptually and empirically, for the rest of the analysis, we utilize pros only.}
%, leaving a more detailed analysis on sustainability mentions in company cons for future work. %\todo{add implications of this.}


\begin{table}
\centering
\begin{tabular}{@{}lrrrr@{}}
\toprule
                          & \multicolumn{2}{l}{\begin{tabular}[c]{@{}l@{}}avg s-BERT \\ similarity\end{tabular}} & \multicolumn{2}{l}{\begin{tabular}[c]{@{}l@{}}proportion of \\ relevant reviews\end{tabular}} \\ \midrule
Goal                      & pros                                      & cons                                     & pros                                          & cons                                          \\ \midrule
Monetary        & 0.234                                     & 0.153                                    & 0.180                                         & 0.202                                         \\
Health                    & 0.185                                     & 0.110                                    & 0.177                                         & 0.084                                         \\
Education                 & 0.194                                     & 0.114                                    & 0.175                                         & 0.112                                         \\
Diversity           & 0.130                                     & 0.080                                    & 0.130                                         & 0.026                                         \\
Infrastructure & 0.163                                     & 0.113                                    & 0.174                                         & 0.084                                         \\
Atmosphere    & 0.157                                     & 0.102                                    & 0.175                                         & 0.058                                         \\ \bottomrule
\end{tabular}
\caption{Average similarity scores for pros and cons based on s-BERT similarity, and the proportion of reviews shortlisted based on our deep learning method for pros and cons.}
\label{tab:pros_vs_cons}
\end{table}


Finally, each review consisted of several sentences where any sentence could be expressing an internal sustainability effort. Therefore, to score each individual pro review $p$ with a relevance score, we considered the score of a review for ISE $i$ to be the highest scored sentence of that review $p$. %\notelc{why so? in case the same review has more than 1 sentence that is relevant to a goal? might need clarification if so.} 
Thus, we selected a set of sustainability-relevant reviews for each of the 13 goals.

\begin{equation}
   sim(p,i)= cosine[ v_p, v_i]
\end{equation}
where p is each post and $i$ is the definition of a UN sustainability goal, $v_p$ is the vector embedding post obtained from s-BERT, and $v_i$ is the vector embedding the UN's definition of the SDG goal counterpart of $i$, also obtained through s-BERT. 

%\notelc{up to now we have not spoken about unit of analysis, this comes later. can we avoid mentioning it now, it is only confusing and i believe not needed until step 3. also, what id def(g)? i guess the UN text/priose definition of g but we do not say and we do not use it consistently - need fix notation in later pass}


Then, our framework \rev{formulates an s-BERT similarity score, $sim_t(v_p,v_i)$, that measures whether and the extent to which a post $p$ is about ISE $i$ with the following function:}

\rev{
\begin{equation}
    sim_t(v_p,v_i) = \begin{cases} sim(v_p,v_i), & \text{if } sim(v_p,v_i)>0.31 \textrm{ AND } sim(v_p,v_i) \textrm{ is in } 95\% percentile
    \\
    0,              & \text{otherwise}
    \end{cases}
\end{equation}
}

\todo{THE FOLLOWING IS INCORRECT/VAGUE. WHERE 0.31 CAME FROM? 95\% of WHICH DISTRIBUTION?} where $p$ is the post, $v_p$ is the vector embedding the post, and  $v_i$ is the vector embedding the UN's definition of practices around $i$. The post is about $i$ if two conditions are met: the post's similarity to $def(i)$ is above a fixed threshold 0.31, and greater than the 95\% similarity value. 


%\begin{equation}
%   label(p,i)= I(sim(v_p,v_i)>0.30 \textrm{ AND } sim(v_p,v_i) \textrm{ is in } 95\%)
%\end{equation}



%where $p$ is the post, $I$ is an indicator function returning 0 ($p \notin i$) or 1 ($p \in i$), $v_p$ is the vector embedding the post, and  $v_i$ is the vector embedding the UN's definition of practices around $i$. The post is about $i$ if two conditions are met: the post's similarity to $def(i)$ is above a fixed threshold 0.30, and greater than the 95\% similarity value. 


% \begin{figure}[ht]
% \centering
% \includegraphics[width=\linewidth]{figs/goal_dist.png}
% \caption{\textbf{Distribution of sentence similarity scores for the different goals.}}
% \label{fig:goal_dist}
% \end{figure}


To understand whether the above method correctly captured mentions of the pre-selected 13 SDGs in the corporate context, three independent annotators manually assessed the five highest ranked sentences for each goal based on their similarity score for that goal. By assessing the top five, we obtained an understanding of the upper bound of our method. Agreement between annotators, measured using Fleiss Kappa, was high (0.83). For disagreements, we used majority rating to obtain a final ground-truth label for relevance. We retained only those goals for which at least 4 of the top 5 highest ranked sentences were relevant to the goal, i.e, they mention concepts related to that goal, for example, mention gender diversity initiatives of the company for the gender equality goal. We found that the goals related to environmental sustainability, `clean water' and `climate action', faced word sense disambiguation issues with shortlisted sentences talking about the different aspects of the \textit{work environment}, for example, the cleanliness of office spaces. For comparison, the highest ranking sentences for the other goals are more precise and thematically related. Thus, we discarded a further 5 UN goals in this step (clean energy, clean water, climate action, responsible consumption, and no poverty) and are left with 8 goals. 

%\subsection*{Aggregating scores at the unit  of analysis and creating a Composite Score}
\subsection*{Step 3 - Consolidation of goals}

Sustainability goals are not mutually exclusive and a certain degree of overlap might be expected (e.g., %\notelc{give an example of a partial, tolerable, overlap - such as training and professional development links to both education and decent work}
Work-life balance facilitates both health and gender equality, and is therefore a concept shared by both ISEs). However, there might be cases where two goals are so strongly related to one another that we cannot discern between the two. To systematically tackle the issue of semantically overlapping goals, we plotted the content overlap of sentences for each pair of the remaining 8 goals, by computing the proportion of sentences that the two goals have in common (Figure~\ref{fig:goal_overlap}):

\rev{
\begin{equation}
    O(i^j, i^k) = \frac{\sum sim_s(v_p, v_i^j) \cap \sum sim_s(v_p, v_i^j)}{\sum sim_s(v_p, v_i^j)}
\end{equation}
}

\noindent Note that $O(i_j, i_k)$ is not a symmetric metric since the total relevant reviews for $i_j$ and $i_k$ need not be the same.

\begin{figure}[!ht]
\centering
\includegraphics[width=\linewidth]{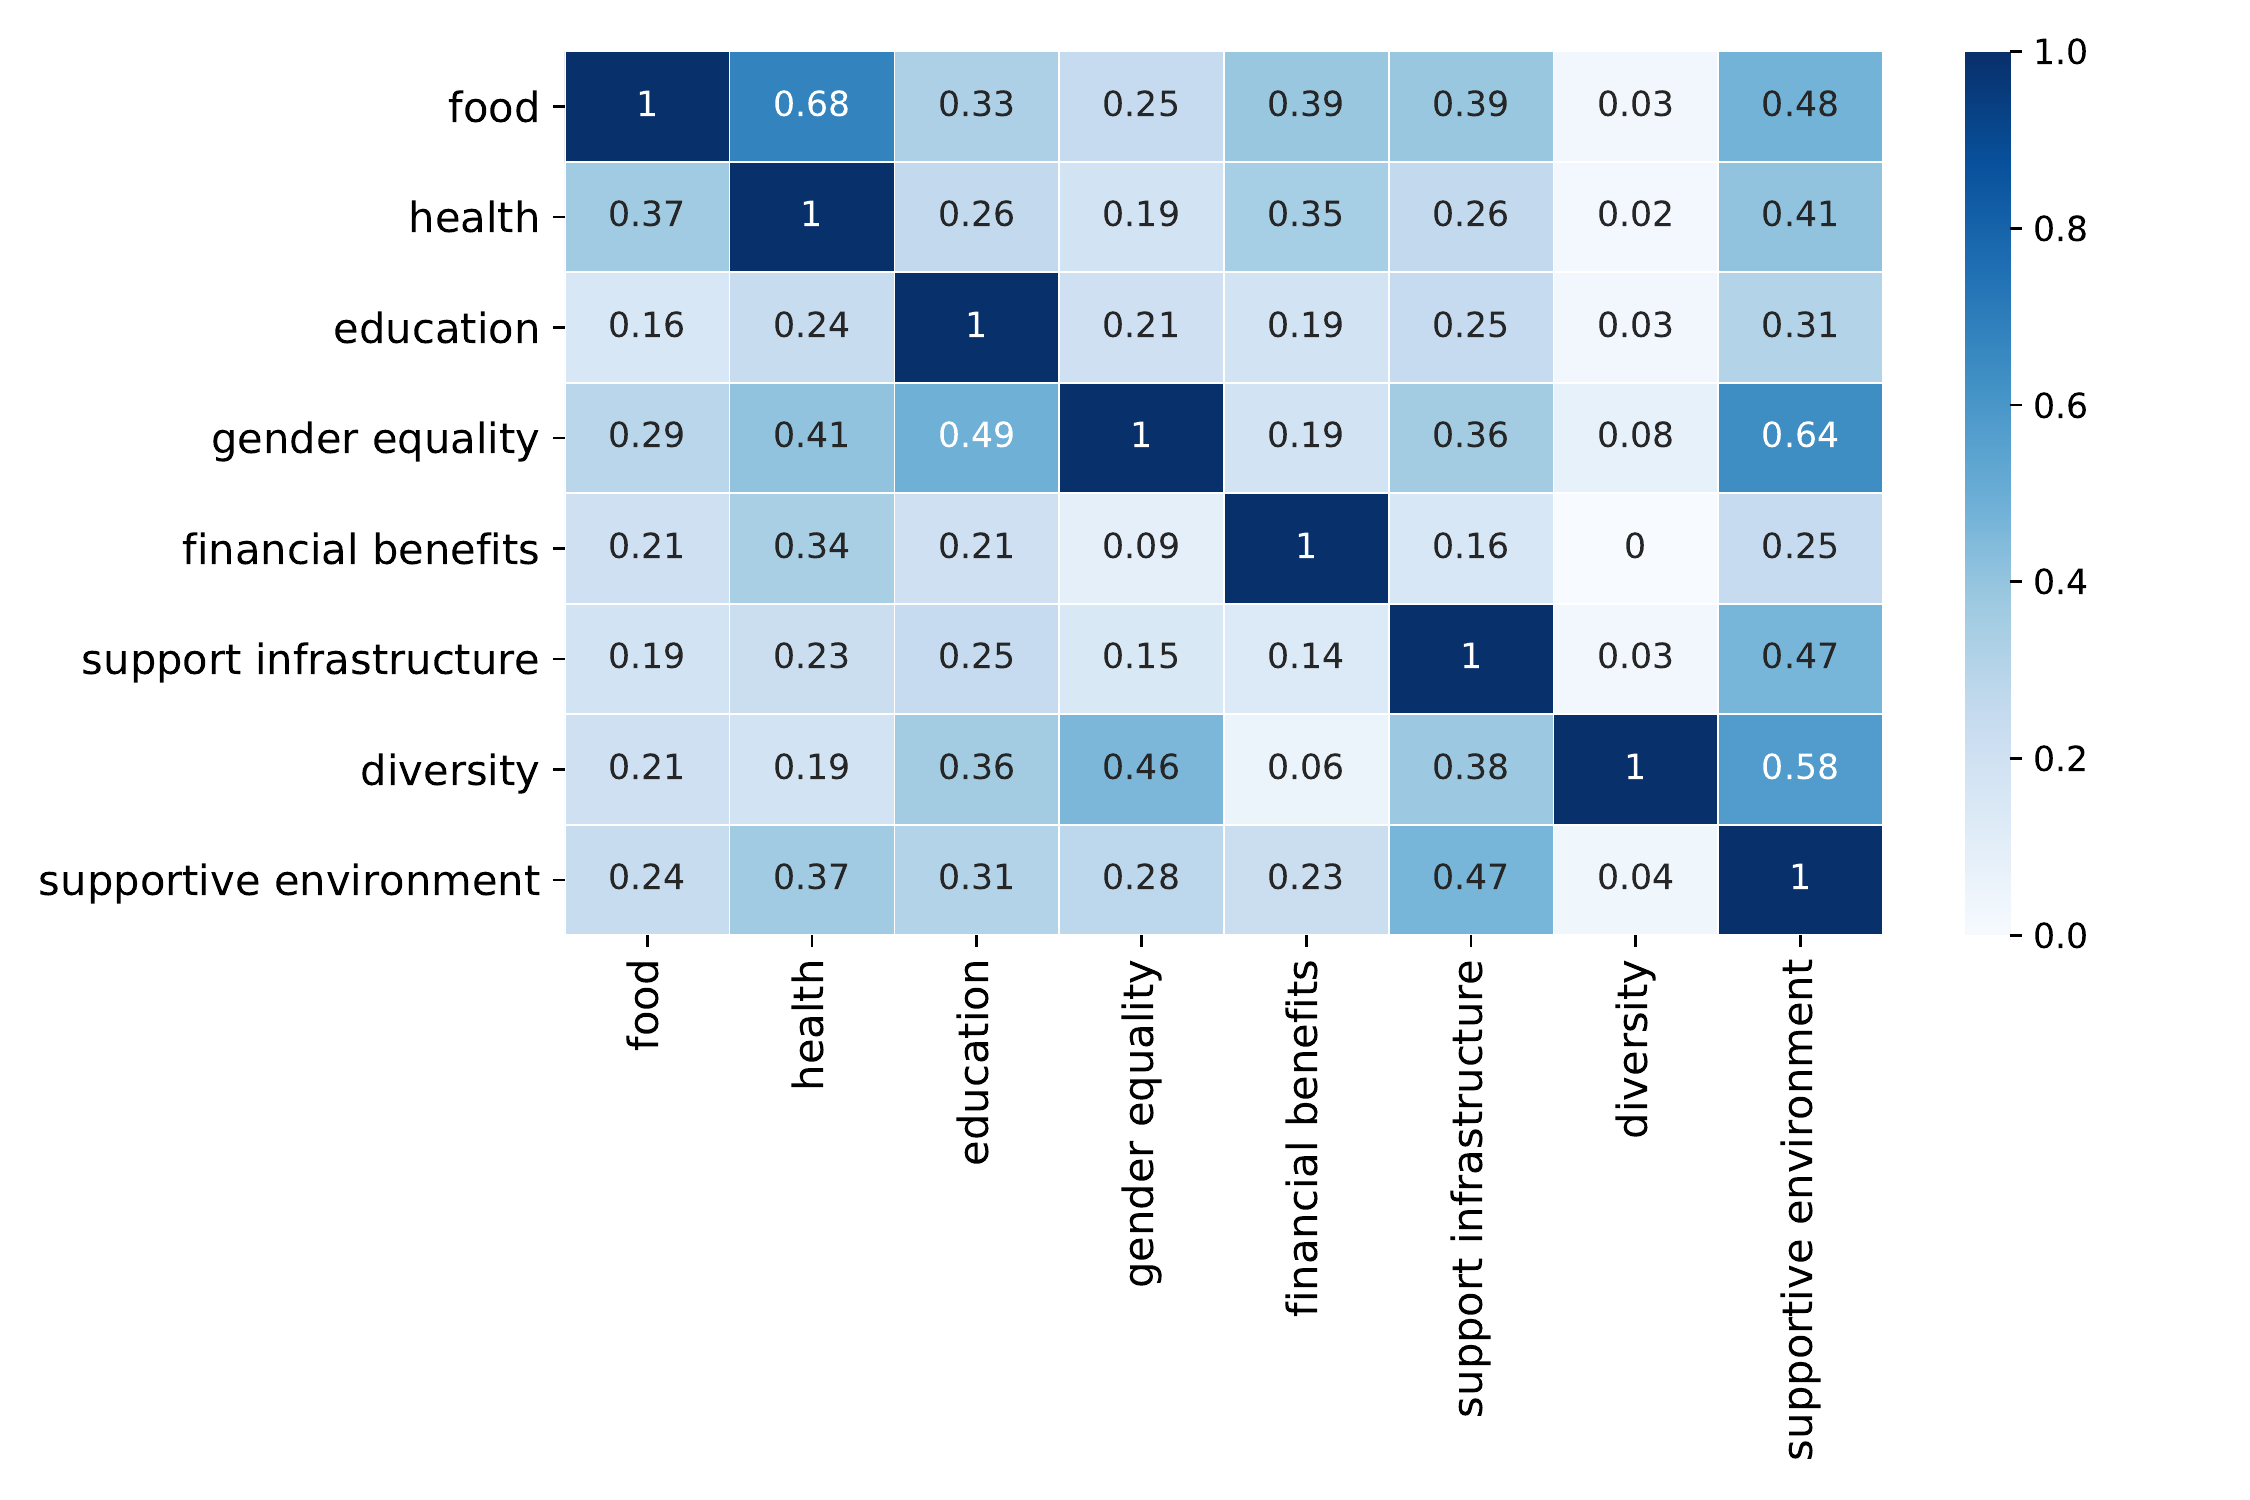}
\caption{Overlap between goal pair. Step 3 of the goal selection process checked for content overlap between each pairs of goals.}
\label{fig:goal_overlap}
\end{figure}

We observe that the only overlap higher than $0.5$ occurs for goals `food (no hunger)' vs `health'. These have indeed strong conceptual relatedness in the corporate sector, and thus proceeded by subsuming `no hunger' under `health'. 

%\notelc{how do we justify the merging of diversity and gender? the overlap is < 0.5 and similar to that of supportive environment and support infrastructure, yet we kept the latter separate. pls check possible explanation below - is that true?}

We note that two other pairs of goals exhibit semantic relatedness close to 0.5: these are `supportive environment' vs `supporting infrastructure', and `diversity' vs `gender equality'. To decide whether to combine or keep these pairs separate, the three annotators qualitatively assessed the top 5 reviews for each goal. They found that `supportive environment' and `supporting infrastructure' to cover related yet different concerns; however, they discovered that goal `diversity' (reducing inequality) was mostly expressed through mentions of `gender discrimination', thus becoming almost indistinguishable from the concerns raised for the other goal `gender equality'. It was decided to also merge these two goals together. 

%\notelc{might be easier to present table with first 2 columns swapped (our goal, the original it was derived from, example)}



We try other variants of the aggregation score. or 

\rev{
\begin{equation*}
    S(u, i) = \frac{\sum_{p \in u}^{N(u,i)} \frac{e^{sim_s(v_p,v_i)}}{e}}{N(u)} 
\end{equation*}
}

or

\rev{
\begin{equation*}
    S(u, i) = \frac{\sum_{p \in u}^{N(u,i)} \frac{log{(sim_s(v_p,v_i)+1)}}{log(2)}}{N(u)} 
\end{equation*}
}


where $R(u, i)$ is the number of  reviews at study unit $u$  relevant to practices around $i$, and $N(u)$ is the total number of  reviews at study unit $u$.






\section{Method Validation}

Here we supplement the results in our main paper on validating our deep learning method for detecting ISEs. 

\mbox{ }\\
\noindent
\subsection*{ISEs and Online Ratings. } Reviewers have the option to rate the companies they are reviewing based on five different facets --- culture, balance, company, management, career, and an overall score. %Figure XX shows the distribution of the different ratings in our dataset. 
After aggregating the ISE scores at a company level, we found the correlation between our six ISE scores with the company's ratings (Table \ref{tab:glassdoor_rating_weighted}). To see whether the correlations are merely an artifact of company popularity, we also found the correlation between the total number of reviews of a company and our 6 scores and the 6 ratings.

The number of company reviews were not correlated with the ratings, while being slightly (but not significantly) correlated with our scores. This indicates that our correlations are indeed capturing the relationship between our scores and the online ratings, rather than capturing overall company popularity. Our health ISE is most strongly correlated with balance $[r = 0.7, p < 0.001]$, possibly since the health ISE captures mentions of work-life balance. The education, gender equality, infrastructure, and supportive environment ISEs are strongly and significantly associated with the career rating. Education and training opportunities as well as infrastructure facilitate career growth~\cite{morgan2017employee}. Financial benefits is most strongly correlated with the overall company rating $[r = 0.75, p < 0.001]$, in line with previous research that found the importance of salary in company evaluations~\cite{cascio2006decency}. Finally, supportive environment is strongly associated with multiple types of ratings, but the ratings for culture and management are most strongly associated with supportive environment out of all the 6 ISEs $[r = 0.71, p < 0.001]$ and $[r = 0.66, p < 0.001]$, respectively, further hinting that our supportive environment ISE captures company management and culture well. 

%Company culture and management is most strongly and highly correlated with our supportive environment score. On the other hand, the balance rating is most strongly correlated with health. As these two dimensions of sustainability are related to company culture and balance, respectively, strong correlations indicates that our method is indeed capturing these dimensions. The other ratings, (career, company, and overall) do not show a particularly discerning correlation with our scores. Career is strongly correlated with education, supportive infrastructure and environment, possibly as education and technically empowered environment facilitates career growth. 

%\comments{Matteo - I would add the r coefficient and p-value also in the text e.g., On the other hand, the balance rating is most strongly correlated with health (r= x.xx; p<x.xx)} 

\begin{table}[!t] 
\centering
\small
\begin{tabular}{llllllll}
\hline
Rating                                                            & Monetary         & Health           & Education        & Diversity        & Infrastructure   & Atmosphere       & \begin{tabular}[c]{@{}l@{}}Total Reviews \\ (logged)\end{tabular} \\ \hline
Culture                                                           & 0.29***          & 0.52***          & 0.57***          & 0.63***          & 0.66***          & 0.71***          & -0.09                                                             \\
Balance                                                           & 0.48***          & \textbf{0.70***} & 0.32***          & 0.56***          & 0.58***          & 0.65***          & -0.15                                                             \\
Management                                                        & 0.26**           & 0.43***          & 0.57***          & 0.62***          & 0.64***          & 0.66***          & -0.06                                                             \\
Career                                                            & 0.40***          & 0.49***          & \textbf{0.70***} & \textbf{0.66***} & \textbf{0.70***} & \textbf{0.72***} & -0.08                                                             \\
Overall                                                           & \textbf{0.75***} & 0.66***          & 0.55***          & 0.61***          & 0.64***          & \textbf{0.72***} & -0.11                                                             \\ \hline
\begin{tabular}[c]{@{}l@{}}Total Reviews \\ (logged)\end{tabular} & -0.15            & -0.29***         & -0.03            & -0.22*           & -0.18            & -0.24*           & 1.00***                                                           \\ \hline
\end{tabular}
\caption{
\textbf{Pearson correlation between overall ratings concerning five aspects on the review platform and our sustainability scores.} The highest correlation with a rating for each ISE is marked in bold. (*** for p < 0.005, ** for p < 0.01, * for p < 0.05) 
%\todo{remove avg rating; keep total reviews as a column BUT add total reviews to the last raw, and, as such, the log(reviews) should be correlated with our six scores}
}
\label{tab:glassdoor_rating_weighted}
\end{table}

\begin{table}[]
\small
\centering
\begin{tabular}{@{}lllll@{}}
\toprule
                  & Gender report & \begin{tabular}[c]{@{}l@{}}Fashion report \\ (Gender Diversity)\end{tabular} & \begin{tabular}[c]{@{}l@{}}Fashion report \\ (Financial Benefit)\end{tabular} & \begin{tabular}[c]{@{}l@{}}Fashion report \\ (Supportive \\ Environment)\end{tabular} \\ \midrule
% unweighted        & 0.257         &                                                                              &                                                                               &                                                                                       \\
$S(u,g)$          & 0.285         & 0.285                                                                             &   0.236                                                                            & 0.246                                                                                      \\
random (baseline) & 0.186         & 0.183                                                                              & 0.185                                                                               & 0.185                                                                                      \\ \bottomrule
\end{tabular}
\caption{Ranked Biased Overlap (RBO) scores measuring the concordance between review-based sustainability rankings and external rankings. Higher RBO scores are better. As a baseline, we compare our rankings against a random ordering of companies (averaged over 1000 runs).}
\label{tab:external_reports}
\end{table}

\begin{table}[]
\small
\centering
\begin{tabular}{@{}cccccc@{}}
\toprule
                  &               & \multicolumn{4}{c}{Fashion Report}                                                                                \\ \midrule
                  & Gender report & Gender Diversity & Financial Benefit & \begin{tabular}[c]{@{}c@{}}Supportive \\ Environment\end{tabular} & Health \\ \midrule
$S(u,g)$          & 0.22          & 0.073            & 0.1               & 0.227                                                             & 0.136  \\
random (baseline) & 0.001         & -0.012           & 0.0008            & -0.015                                                            & 0.002  \\ \bottomrule
\end{tabular}
\caption{Spearman rank correlation measuring the overlap between review-based sustainability rankings and external rankings. As a baseline, we compare our rankings against a random ordering of companies (averaged over 1000 runs).}
\label{tab:external_reports_spearmanr}
\end{table}


% \begin{table}[]
% \centering
% \small
% \begin{tabular}{@{}lllllll@{}}
% \toprule
% variable                          & \begin{tabular}[c]{@{}l@{}}health\\ \end{tabular} & \begin{tabular}[c]{@{}l@{}}education\\\end{tabular} & \begin{tabular}[c]{@{}l@{}}gender diversity\\\end{tabular} & \begin{tabular}[c]{@{}l@{}}financial\\ benefits\end{tabular} & \begin{tabular}[c]{@{}l@{}}infrastructure\\ \end{tabular} & \begin{tabular}[c]{@{}l@{}}supportive\\ environment \end{tabular} \\ \midrule
% P\_3c\_giniCoefficient            & -0.24*                                                               & -0.25*                                                       &                                                                                & \textbf{-0.53***}                                                                         &                                                                                    &                                                                                          \\
% \midrule
% P\_4b\_cultural tightness         & -0.21*                                                               &                                                              &                                                                                &                                                                                  & -0.31*                                                                             & -0.24*                                                                                   \\ \midrule
% P\_6b\_politicsNeighbors          & 0.29*                                                                &                                                              & 0.29*                                                                          &                                                                                  &                                                                                    &                                                                                          \\ \midrule
% P\_6h\_politicsBoycott            & 0.29*                                                                &                                                              &                                                                                &                                                                                  &                                                                                    &                                                                                          \\ \midrule
% E\_1e\_occupationsInvestigative   & 0.31*                                                                &                                                              &                                                                                &                                                                                  & 0.34*                                                                              & 0.32*                                                                                    \\ \midrule
% E\_1f\_occupationsRealistic       & -0.26*                                                               &                                                              & -0.23*                                                                         & 0.33*                                                                            & \textbf{-0.45***}                                                                           & -0.29*                                                                                   \\ \midrule
% E\_2a\_gdp                        & 0.29*                                                                & 0.36*                                                        & 0.36*                                                                          &                                                                                  & 0.30*                                                                              & \textbf{0.46***}                                                                        \\ \midrule
% S\_1b\_lgbtqTravelIndex           & 0.37**                                                               &                                                              & 0.35*                                                                          &                                                                                  & \textbf{0.49***}                                                                            & 0.33*                                                                                    \\ \midrule
% S\_2a\_collectivism               & -0.22*                                                               & -0.22*                                                       &                                                                                & -0.31*                                                                           &                                                                                    &                                                                                          \\ \midrule
% S\_6b\_religiousModerately        & -0.26*                                                               & -0.21*                                                       &                                                                                & -0.39**                                                                          & -0.26*                                                                             &                                                                                          \\ \midrule
% S\_9a\_urbanPop                   & 0.35*                                                                &                                                              &                                                                                &                                                                                  &                                                                                    & 0.35*                                                                                    \\ \midrule
% S\_9b\_fiveThirtyEightUrbanIndex  & 0.30*                                                                &                                                              &                                                                                & -0.27*                                                                           & 0.39**                                                                             & 0.31*                                                                                    \\ \midrule
% Creativity Index                  & 0.34*                                                                &                                                              &                                                                                & -0.24*                                                                           & \textbf{0.52***}                                                                            & 0.38**                                                                                   \\ \midrule
% P\_6i\_politicsGroup              &                                                                      & 0.30*                                                        &                                                                                & 0.31*                                                                            &                                                                                    &                                                                                          \\ \midrule
% S\_5a\_violentCrimes              &                                                                      & -0.31*                                                       &                                                                                &                                                                                  & -0.39**                                                                            &                                                                                          \\ \midrule
% population\_2019                  &                                                                      &                                                              &                                                                                & -0.32*                                                                           &                                                                                    &                                                                                          \\ \midrule
% population\_2019\_log             &                                                                      &                                                              &                                                                                & \textbf{-0.40***}                                                                         &                                                                                    &                                                                                          \\ \midrule
% P\_1a\_foreignBorn                &                                                                      &                                                              &                                                                                & -0.24*                                                                           & 0.30*                                                                              &                                                                                          \\ \midrule
% P\_1b\_hateCrimes                 &                                                                      &                                                              &                                                                                & -0.28*                                                                           &                                                                                    &                                                                                          \\ \midrule
% P\_3a\_stateEqualityRanking       &                                                                      &                                                              &                                                                                & 0.29*                                                                            &                                                                                    &                                                                                          \\ \midrule
% P\_4a\_empLawEnforcement          &                                                                      &                                                              &                                                                                & -0.34*                                                                           &                                                                                    &                                                                                          \\ \midrule
% P\_4c\_horizontalLegalRestriction &                                                                      &                                                              &                                                                                & -0.21*                                                                           & 0.30*                                                                              &                                                                                          \\ \midrule
% P\_5a\_republican                 &                                                                      &                                                              &                                                                                & \textbf{0.41***}                                                                          & -0.38**                                                                            &                                                                                          \\ \midrule
% P\_6g\_politicsOfficial           &                                                                      &                                                              &                                                                                & 0.29*                                                                            &                                                                                    &                                                                                          \\ \midrule
% E\_1a\_occupationArtistic         &                                                                      &                                                              &                                                                                & -0.24*                                                                           & 0.32*                                                                              &                                                                                          \\ \midrule
% E\_1b\_occupationEnterprising     &                                                                      &                                                              &                                                                                & -0.21*                                                                           & \textbf{0.46***}                                                                            & 0.32*                                                                                    \\ \midrule
% S\_3b\_volunteersHours            &                                                                      &                                                              &                                                                                & 0.29*                                                                            &                                                                                    &                                                                                          \\ \midrule
% S\_8a\_educBachelor               &                                                                      &                                                              &                                                                                & -0.20*                                                                           & \textbf{0.42***}                                                                            & 0.29*                                                                                    \\ \midrule
% total reviews                     &                                                                      &                                                              &                                                                                & -0.29*                                                                           & 0.28*                                                                              &                                                                                          \\ \midrule
% P\_2a\_freedomIndex               &                                                                      &                                                              &                                                                                &                                                                                  & -0.21*                                                                             &                                                                                          \\ \midrule
% P\_3b\_verticalLegalRestriction   &                                                                      &                                                              &                                                                                &                                                                                  & -0.36*                                                                             &                                                                                          \\ \midrule
% E\_3e\_economicFreedomIndex       &                                                                      &                                                              &                                                                                &                                                                                  & -0.21*                                                                             &                                                                                          \\ \midrule
% S\_1a\_lgbtqEquality              &                                                                      &                                                              &                                                                                &                                                                                  & \textbf{0.42***}                                                                            &                                                                                          \\ \midrule
% S\_4c\_charitableContributions    &                                                                      &                                                              &                                                                                &                                                                                  & -0.24*                                                                             &                                                                                          \\ \midrule
% S\_6a\_religiousVery              &                                                                      &                                                              &                                                                                &                                                                                  & -0.27*                                                                             &                                                                                          \\ \midrule
% S\_6c\_religiousNon               &                                                                      &                                                              &                                                                                &                                                                                  & 0.32*                                                                              &                                                                                          \\ \bottomrule
% \end{tabular}
% \caption{Significantly correlated variables with the different goals ($^{*}$p$<$0.05; $^{**}$p$<$0.01; $^{***}$p$<$0.005)}
% \label{tab:state_control}
% \end{table}

\mbox{ }\\
\noindent
\subsection*{ISEs and external reports.} We used external sustainability reports to assess validity further. Reports on sustainability are few and fragmented\cite{burritt2010sustainability}, making it challenging to establish validity through external reports. However, we obtained two external reports on sustainability and compared the ranking of companies in them with our review-based ISE rankings, finding that our method substantially outperforms a random baseline. Specifically, we utilized two reports --- (1) one on gender diversity indicators of S\&P 500 companies\cite{equileap} providing a ranking of 25 companies performing strongly in terms of gender equality (called gender report from now on), and (2) the Fashion Transparency Index~\cite{fti}, that scores companies in the fashion sector on different sustainability metrics such as `Discrimination' and `Diversity and Inclusion' (called the fashion report from now on). For the gender report, we have 13 companies with common out of the 25, while for the Fashion Transparency Index, we have 12 companies in common with our reviews datasets. %\comments {Matteo - I could not understand this sentence}. 
%\comments{Matteo - should methodological details be written the past tense? Can we be more specific and include title and citations for both reports? e.g., we talk about the fashion report but the title is "Fashion Transparency Index - I have changed the parts on the Fashion Transparency Index but I don't know the title of the other report}

We used our goal-specific ISE metric $S(u, i)$ to rank companies based on their sustainability scores for each of the 6 goals and obtain 6 lists of ranks --- $R^i_g$, where $i$ stands for \textbf{internal rankings}. To compare these ranks with the external reports, we need a ranked list of companies from the gender and Fashion Transparency Index report. For the gender report, we simply used the rankings provided in the report ($R^G_{gender}$ where $G$ stands for the gender report) 
%\notelc{don't understand notation - what is G vs gender?} 
which we compared with $R^i_{gender}$. The Fashion Transparency Index report, on the other hand, does not provide an explicit ranking of companies but scores them either 0 or 0.5 for different metrics. To convert these scores to rankings comparable with our sustainability rankings, three annotator's first mapped the 21 metrics in the Fashion Transparency Index report to our 6 goals to obtain sub-facets of our 6 goals (the mapping can be found in Table~\ref{tab:fti_mapping}). For example, `gender equality' is comprised of the metrics `Discrimination', `Diversity and Inclusion', `Equal Pay', `Harassment and Violence', and, `Maternity Rights and Parental Leave'. The annotators had one disagreement (`working hours' belonging to `gender equality') which was resolved after a round of discussions. Based on this mapping, we averaged the scores of a company on different sub-facets and obtain an external score for each goal $g$. We then ranked the companies based on this score to obtain an external ranking for $g$, namely, $R^F_g$ (where $F$ stands for fashion report). We then compared $R^i_g$ with $R^F_g$.

Since the ranked lists might have different companies, we utilized a measure called `rank biased overlap' (RBO) which was designed for measuring the goodness of ranking between non-overlapping ranked lists~\cite{webber2010similarity} (Table \ref{tab:external_reports}). RBO scores lie between 0 and 1, with a higher score representing better concordance between lists. We also find the Spearman correlation between the ranking of the companies that are common in both lists (Table \ref{tab:external_reports_spearmanr}). Note that $s(u, i)$ outperforms the random baseline for both the gender report and fashion report categories.


\section*{Distribution of Similarity Score}

\begin{figure*}[!t]
    \centering
    \includegraphics[width=\linewidth]{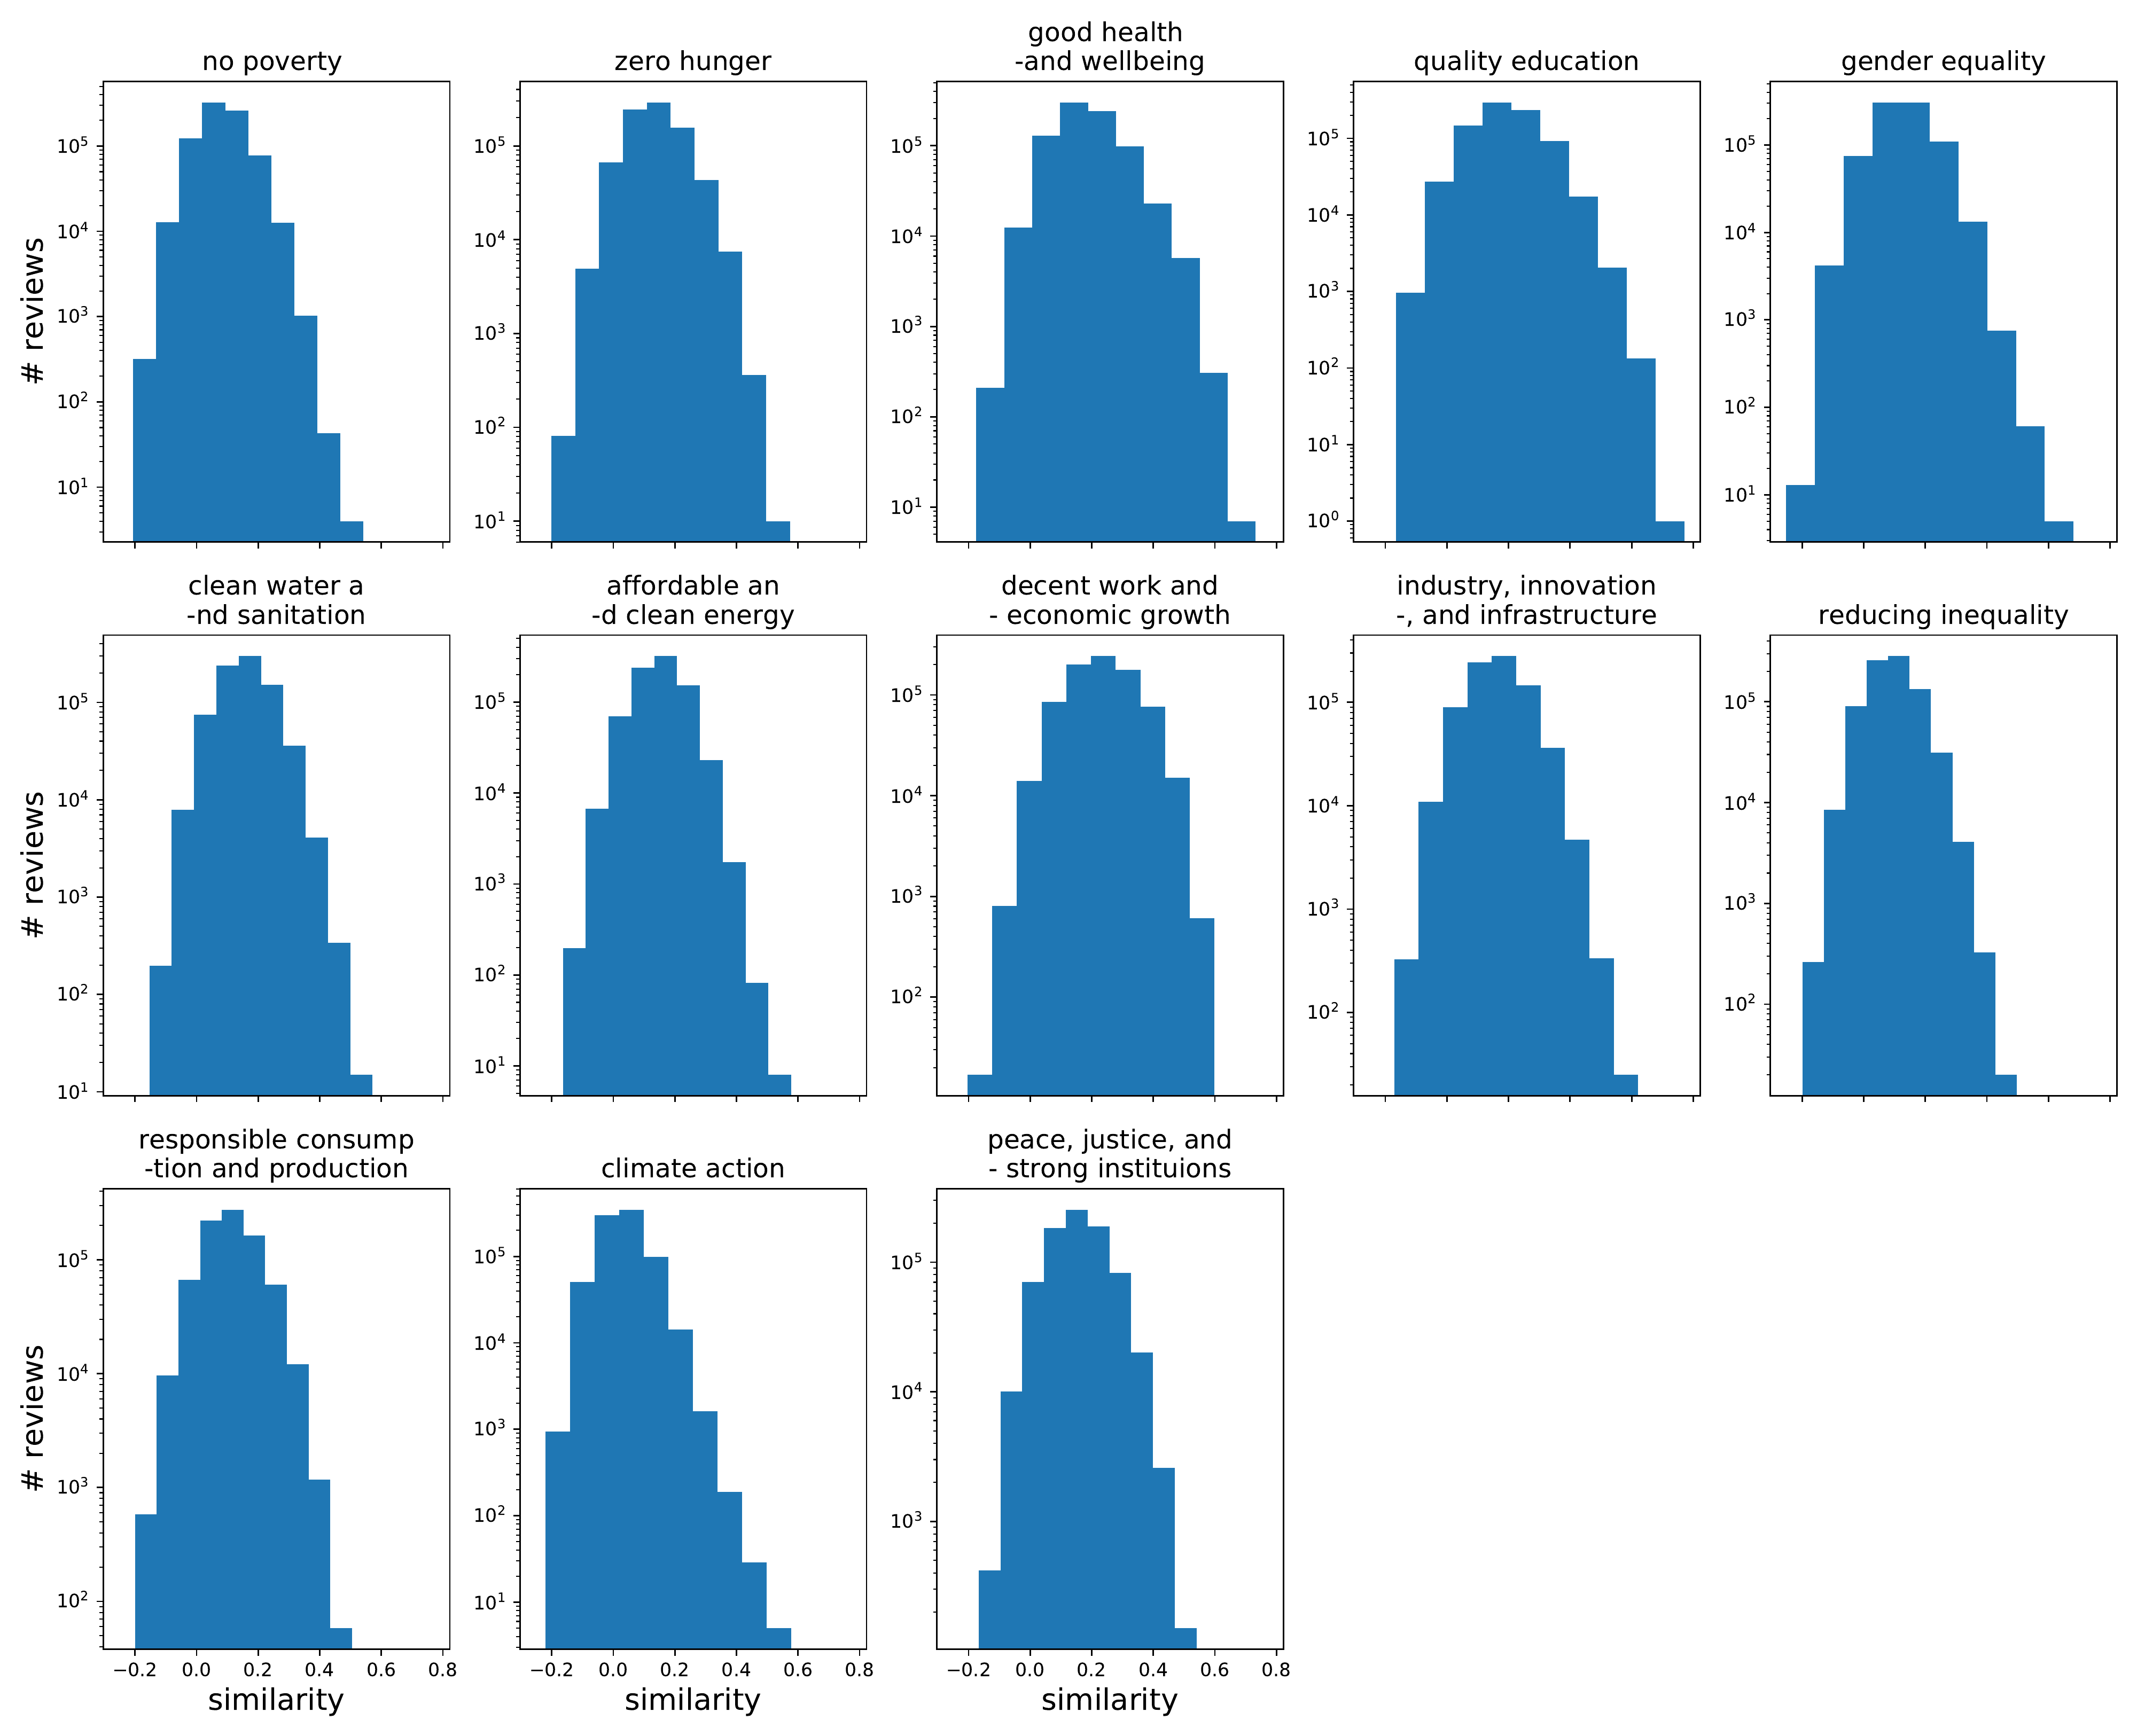}
    \caption{The distribtion of similarity scores for all 13 SDGs shortlisted after the conceptual check.}
    \label{fig:sim_dist}
\end{figure*}

\clearpage

\section*{Stock Analysis}

\textcolor{blue}{The geometric mean of stock growth is calculated as, $GM({\textrm{stock growth}_{[09-19]}}) = \Pi (\textrm{stock growth}_{[09-19]}(c))^{1/n} $, where $c$ is a company in a specific \emph{(ISE type, percentile)} bin, and $n$ is the number of the companies in such a bin.}


\begin{comment}

\section*{How did ISEs evolve over time?}

\begin{figure}[t]
\centering
\includegraphics[width=\linewidth]{figs/financial_vs_non_financial.pdf}
\caption{\textbf{Change in the fraction of reviews related to different ISEs over time.}}
\label{fig:temporal_distribution}
\end{figure}

We assess the growth is different types of ISEs over time in the platform reviews (Figure~\ref{fig:temporal_distribution}). We note that while reviews discussing financial benefits, gender equality, and health have grown over time. However, in terms of growth, we see that financial benefits ISEs, despite being a regular concern, plateau over time. Reviews discussing gender equality and health, on the other hand, grow at a more rapid pace after 2014, indicating that these may be more emerging sustainability concerns from employees. The other goals like education and infrastructure either reduce over time or stay stable.

\textcolor{blue}{The trajectory of ISEs can be mapped to offline events such as the economic recession of 2009 and high-profile scandals on occupational sexism~\cite{pao}. Note that financial benefits ISEs continued to rise before 2015, with employee reviews praising companies for pay and salary benefits, possibly a byproduct of economic recovery. However, financial ISEs start to plateau around 2015, while the US economy underwent a slowdown~\cite{slowdown}. In 2015, there were several lawsuits against companies, alleging gender discrimination in the work place and casting grater scrutiny on gender diversity and equality practices of companies~\cite{pao}.}

\end{comment}

\section*{US State Analysis}

\subsection*{PCA for ISEs on a state level}

To complement the company level PCA in the main paper, we also include the state-level PCA. We found that the first two components explained 74\% and 14\% of the variance in the data, while also showing that financial benefits are orthogonal to the other ISEs.

\begin{table}[]
\begin{tabular}{llrrrrrrr}
\hline
               & Monetary & Health & Education & Diversity & Infrastructure & Atmosphere & PC1           & PC2           \\ \hline
Monetary       & 1.00     & 0.59   & 0.49      & 0.54      & 0.22           & 0.48       & \textbf{0.61} & \textbf{0.77} \\
Health         & 0.59     & 1.00   & 0.65      & 0.84      & 0.75           & 0.86       & 0.92          & 0.06          \\
Education      & 0.49     & 0.65   & 1.00      & 0.81      & 0.69           & 0.79       & 0.86          & -0.03         \\
Diversity      & 0.54     & 0.84   & 0.81      & 1.00      & 0.76           & 0.88       & 0.95          & -0.02         \\
Infrastructure & 0.22     & 0.75   & 0.69      & 0.76      & 1.00           & 0.82       & 0.84          & -0.45         \\
Atmosphere     & 0.48     & 0.86   & 0.79      & 0.88      & 0.82           & 1.00       & 0.95          & -0.12         \\
PC1            & 0.61     & 0.92   & 0.86      & 0.95      & 0.84           & 0.95       & 1.00          & -0.00         \\
PC2            & 0.77     & 0.06   & -0.03     & -0.02     & -0.45          & -0.12      & -0.00         & 1.00          \\ \hline
\end{tabular}
\caption{State level PCA cross-correlation where, like at company level, we found the two facets of ISEs as well.}
\label{state_pca}
\end{table}

\subsection*{Cross-Correlation between ISEs and Socioeconomic Indicators}

\begin{table}[!h]
\centering
\scriptsize
\begin{tabular}{@{}lllllllllll@{}}
\toprule
                                                                  & Wealth  & Inequality & Creativity & Urban Population & Health  & Education & 
                             Diversity & 
                             Monetary & 
                             Infrastructure & 
                             Atmosphere \\ \midrule
Wealth                                                            & 1.00*** & 0.03       & 0.50***    & 0.48***      & 0.30*   & 0.35*     & 0.37**                                                     & 0.07                                                          & 0.30*                                                             & 0.46***                                                            \\
Inequality                                                        & 0.03    & 1.00***    & 0.35*      & 0.23         & -0.21   & -0.24     & -0.17                                                      & -0.55***                                                      & -0.04                                                             & -0.16                                                             \\
Creativity                                                        & 0.50*** & 0.35*      & 1.00***    & 0.66***      & 0.36*   & 0.22      & 0.26                                                       & -0.25                                                         & 0.52***                                                           & 0.37**                                                            \\
Urban Population                                                      & 0.48*** & 0.23       & 0.66***    & 1.00***      & 0.36*   & 0.16      & 0.26                                                       & -0.05                                                         & 0.27                                                              & 0.36*                                                             \\
Health                                                            & 0.30*   & -0.21      & 0.36*      & 0.36*        & 1.00*** & 0.74***   & 0.86***                                                    & 0.59***                                                       & 0.78***                                                           & 0.87***                                                           \\
Education                                                         & 0.35*   & -0.24      & 0.22       & 0.16         & 0.74*** & 1.00***   & 0.82***                                                    & 0.58***                                                       & 0.69***                                                           & 0.80***                                                           \\
\begin{tabular}[c]{@{}l@{}}gender \\ equality\end{tabular}        & 0.37**  & -0.17      & 0.26       & 0.26         & 0.86*** & 0.82***   & 1.00***                                                    & 0.56***                                                       & 0.75***                                                           & 0.87***                                 \\
\begin{tabular}[c]{@{}l@{}}financial \\ benefits\end{tabular}     & 0.07    & -0.55***   & -0.25      & -0.05        & 0.59*** & 0.58***   & 0.56***                                                    & 1.00***                                                       & 0.27                                                              & 0.51***                                        \\
\begin{tabular}[c]{@{}l@{}}supporting \\ infrastructure\end{tabular} & 0.30*   & -0.04      & 0.52***    & 0.27         & 0.78*** & 0.69***   & 0.75***                                                    & 0.27                                                          & 1.00***                                                           & 0.81***                                      \\
\begin{tabular}[c]{@{}l@{}}supportive\\ environment\end{tabular}  & 0.46*** & -0.16      & 0.37**     & 0.36*        & 0.87*** & 0.80***   & 0.87***                                                    & 0.51***                                                       & 0.81***                                                           & 1.00***                                        \\
% composite                                                         & 0.36*   & -0.26      & 0.28*      & 0.26         & 0.93*** & 0.89***   & 0.94***                                                    & 0.68***                                                       & 0.83***                                                           & 0.94***                                                           & 1.00***   \\ 
\bottomrule
\end{tabular}
\caption{Cross-correlation matrix between the three state socioeconomic variables (wealth, gini, and creativity) and the ISEs ($^{*}$p$<$0.05; $^{**}$p$<$0.01; $^{***}$p$<$0.005)
}
\label{tab:state_cross_correlation}
\end{table}

\textbf{Pairwise correlations.} Table~\ref{tab:state_cross_correlation} reports the pairwise correlations among all our variables: each of the six $S(u,i)$, wealth, inequality and the creativity index.  

\begin{comment}

\comments{Indira: I think we don't need the rank difference map anymore}
\subsection*{Spatial Distribution of Emerging Sustainability}

\begin{figure*}[!t]
    \centering
    \includegraphics[width=\linewidth]{supplementary/figure/rank_diff_USA.pdf}
    \caption{We plot the difference between the PCA 1 rank and the PCA 2 rank of states. Recall that PCA 1 is the emerging dimension of sustainability while PCA 2 is the traditional dimension (financial benefits). The rank difference metric ranges between -50 to 50, where lower values signify higher scores for emerging sustainability efforts (like CA, MN), while scores close to zero signify equal efforts in both facets of sustainability (OK, UT), and finally high scoring states on rank diff are those that score highly in the financial facets of sustainability and lower on the emerging ones (MT, ND). %\todo{do we need this?}
    }
    \label{fig:rank_diff}
\end{figure*}
\end{comment}

\begin{figure*}[!t]
    \centering
    \includegraphics[width=\linewidth]{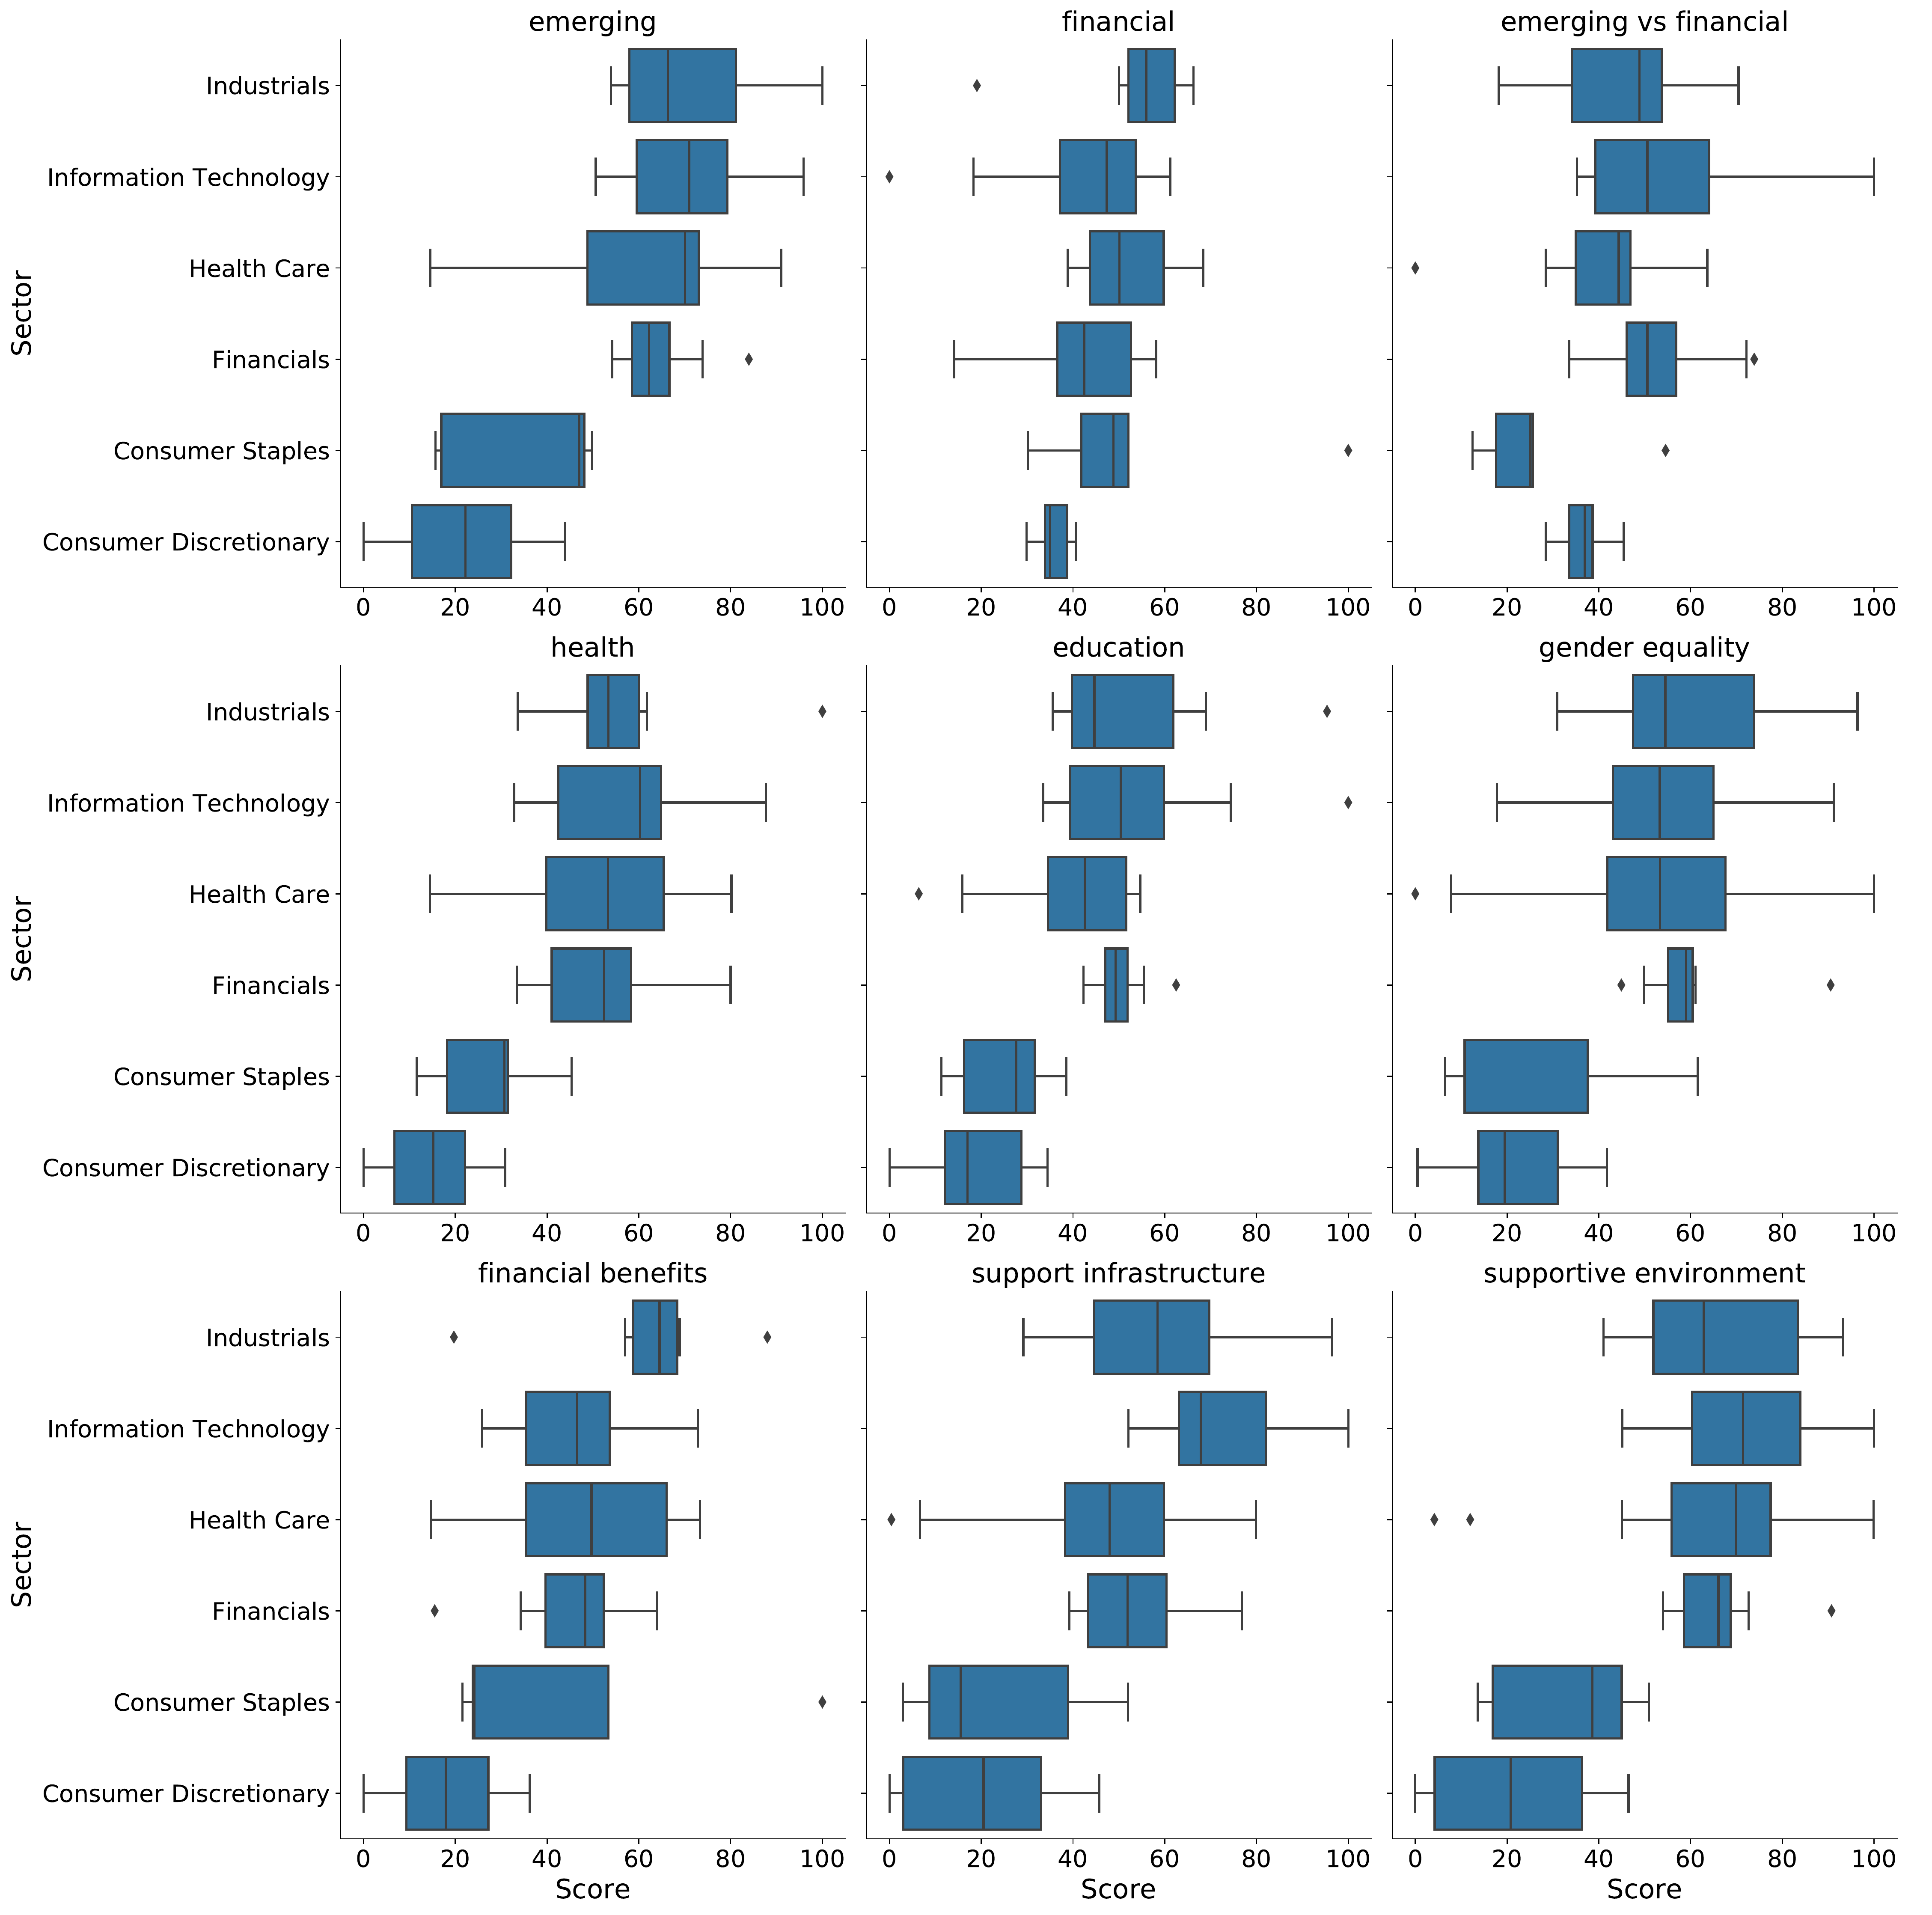}
    \caption{Sustainability scores across different sectors.}
    \label{fig:sector_all}
\end{figure*}


% Please add the following required packages to your document preamble:
% \usepackage{booktabs}
\begin{table}[]
\centering
\scriptsize
\begin{tabular}{@{}lllll@{}}
\toprule
Fashion Report Metric                                                                                                       & NLP ISE 1              & NLP ISE 2          & NLP ISE 3          & NLP ISE 4       \\ \midrule
Animal Welfare                                                                                                              &                        &                    &                    &                 \\
Annual Leave \& Public Holidays                                                                                             & supportive environment & financial benefits &                    &                 \\
\begin{tabular}[c]{@{}l@{}}Anti-bribery, Corruption, \& \\ Presentation of False Information\end{tabular}                   &                        &                    &                    &                 \\
Biodiversity \& Conservation                                                                                                &                        &                    &                    &                 \\
Community Engagement                                                                                                        & supportive environment &                    &                    &                 \\
Contracts \& Terms of Employment                                                                                            & financial benefits     &                    &                    &                 \\
Discrimination                                                                                                              & gender equality        &                    &                    &                 \\
Diversity \& Inclusion                                                                                                      & gender equality        &                    &                    &                 \\
Energy \& Carbon Emissions                                                                                                  &                        &                    &                    &                 \\
Equal Pay                                                                                                                   & gender equality        & financial benefits &                    &                 \\
\begin{tabular}[c]{@{}l@{}}Freedom of Association, Right \\ to Organise \& Collective Bargaining\end{tabular}               & supportive environment &                    &                    &                 \\
Harassment \& Violence                                                                                  & gender equality        &                    &                    &                 \\
Health \& Safety                                                                                                            & health                 &                    &                    &                 \\
Maternity Rights \& Parental Leave                                                                                          & gender equality        &                    &                    &                 \\
Notice Period, Dismissal \& Disciplinary Action                                                                             & supportive environment &                    &                    &                 \\
Restricted Substances List                                                                                                  &                        &                    &                    &                 \\
\begin{tabular}[c]{@{}l@{}}Wages \& Financial Benefits \\ (e.g. bonuses, insurance, social security, pensions)\end{tabular} & financial benefits     &                    &                    &                 \\
Waste \& Recycling (Packaging/Office/Retail)                                                                                &                        &                    &                    &                 \\
Waste \& Recycling (Product/Textiles)                                                                                       &                        &                    &                    &                 \\
Water Usage \& Footprint                                                                                                    &                        &                    &                    &                 \\
Working Hours \& Rest Breaks                                                                                                & supportive environment & health             & financial benefits & gender equality \\ \bottomrule
\end{tabular}
\label{tab:fti_mapping}
\caption{Mapping between fashion report metrics~\cite{fti} and our 6 ISEs. Note that some metrics are applicable for multiple goals.}
\end{table}


\clearpage
\bibliographystyle{plain}
\bibliography{supplementary}

\end{document}
